# Supplementary material for: Representation Learning of Tangled Key-Value Sequence Data for Early Classification
Source: arXiv:2404.07454 source file (2024-04-11)
Supplement: Supplementary file 1 [file appendix.tex]

\section{APPENDIX}
\subsection{Expanded dataset descriptions}
